# Supplementary material for: Deep Learning For Time Series Analysis With Application On Human Motion
Source: arXiv:2502.19364 source file (2025-02-26)
Supplement: Supplementary file 1 [file AppendixA.tex]

%----------------------------------------------------------------------------------------
%
% Appendix A
%
%----------------------------------------------------------------------------------------
\chapter[Titre de l'annexe A blablabla]{Titre de l'annexe A blablabla}
\label{appendixA:blablabla}
